# Supplementary material for: Learning High-level Semantic-Relational Concepts for SLAM
Source: arXiv:2310.00401 source file (2024-03-22)
Supplement: Supplementary file 1 [file Appendix.tex]

\section{Appendix}
\label{Appendix}

%%%%
\begin{algorithm}[t]

\caption{\textit{same Room} edge clustering}\label{alg:edge_clustering}
\textbf{Input}: \textit{wall surface} nodes and \textit{same room} edges graph $\mathcal{G}_{WS}$\\
\textbf{Output}: Clustering as list of node lists $\boldsymbol{\mathcal{V}_R}$ \\
\SetKwFunction{FMain}{visit($v_f$)}
\hrulefill \\
$\boldsymbol{\mathcal{V}_R} \gets []$\\
\For{$l_i \in \boldsymbol{N}_{WS}$}{
    $\boldsymbol{\mathcal{E}_{c}} \gets find\_cycles\_of\_size\_l(\mathcal{G}_{WS}, l_i)$\\
    $\boldsymbol{\mathcal{V}_{ini}} \gets \mathcal{E}_{c,j}.nodes \ \forall \ \mathcal{E}_{c,j} \in \boldsymbol{\mathcal{E}_{c}}$\\
    $\mathcal{I}_{count} \gets count\_set\_repetitions(\boldsymbol{\mathcal{V}_{ini}})$\\
    $\boldsymbol{\mathcal{V}_{sort}} \gets sort\_descendent(\boldsymbol{\mathcal{V}_{ini}}, \mathcal{I}_{count})$\\

    \For{$\mathcal{V}_{sort,j} \in \boldsymbol{\mathcal{V}_{sort}}$}{
        \If{$ all(\mathcal{V}_{sort,j} \notin \boldsymbol{\mathcal{V}_R})$}{
        $\boldsymbol{\mathcal{V}_R}.append(\mathcal{V}_{sort,j})$\\
        $\mathcal{G}_{WS}.remove(\mathcal{V}_{sort,j})$\\
        }
        }
}

\end{algorithm}

%%%
